# Supplementary material for: PROVEN: Certifying Robustness of Neural Networks with a Probabilistic Approach
Source: arXiv:1812.08329 source file (2019-01-07)
Supplement: Supplementary file 1 [file appendix.tex]

\appendix
\newpage
\onecolumn

  \vbox{%S
    \hsize\textwidth
    \linewidth\hsize
    \vskip 0.1in
  \hrule height 4pt
  \vskip 0.25in
  \vskip -5.5pt%
  \centering
    {\Large\bf{Certifying Robustness of Neural Networks: A probabilistic approach \\
			Supplementary Material} \par}
      \vskip 0.29in
  \vskip -5.5pt
  \hrule height 1pt
  \vskip 0.09in%
    
  \vskip 0.2in
    
  }
\section{Additional results}

\begin{table*}[h!]
\centering
\caption{Average 10 images with random target, $p = \infty$, ReLU activation, $n$ = number of layers, $m$ = number of nodes in each layer. $\eta = 10^{-6}$ }
\label{tab:different_inputs}
\begin{subtable}{1\textwidth}
\caption{Input is Gaussian i.i.d.}
\label{subtab:gaussianIID}
\begin{tabular}{c|ccccccc|c}
\hline
Indpdt. input $X_i$ & \multirow{2}{*}{$\epsilon_{\text{worst-case}}$} & \multirow{2}{*}{(100 - $\eta$)\% $^\dagger$}  & \multirow{2}{*}{75\%}    & \multirow{2}{*}{50\%}    & \multirow{2}{*}{25\%}    & \multirow{2}{*}{5\%}     & \multirow{2}{*}{0\%}     & improvement$^\dagger$ \\
Model  &  &  &  &  &  &  & & over $\epsilon_{\text{worst-case}}$ \\
\hline
% MNIST 2$\times${[}20{]}   &     &     &     &    &     &        &    & \\
% MNIST 3$\times${[}20{]}   &     &     &     &    &     &        &    & \\
MNIST 2x{[}1024{]} & 0.02904               & \bf 0.03679 & 0.03815 & 0.03828 & 0.03840 & 0.03858 & 0.04075 & \bf 26.6\%\\
MNIST 3x{[}1024{]} & 0.02082               & \bf 0.02287 & 0.02319 & 0.02322 & 0.02324 & 0.02328 & 0.02410 & \bf 9.8 \%\\
MNIST 4x{[}1024{]} & 0.00796               & \bf 0.00816 & 0.00819 & 0.00819 & 0.00819 & 0.00819 & 0.00835 & \bf 2.5 \%\\
% CIFAR 5$\times${[}2048{]}   &     &     &     &    &     &        &    & \\
% CIFAR 7$\times${[}1024{]}   &     &     &     &    &     &        &    & \\
\hline
\end{tabular}
\vspace{0.4cm}
\end{subtable}
\vspace{0.4cm}
\begin{subtable}{1\textwidth}
\caption{Input is \textcolor{blue}{positive} correlated Gaussian}
\label{subtab:gaussianCORR}
\begin{tabular}{c|ccccccc|c}
\hline
Indpdt. input $X_i$ & \multirow{2}{*}{$\epsilon_{\text{worst-case}}$} & \multirow{2}{*}{(100 - $\eta$)\% $^\dagger$}  & \multirow{2}{*}{75\%}    & \multirow{2}{*}{50\%}    & \multirow{2}{*}{25\%}    & \multirow{2}{*}{5\%}     & \multirow{2}{*}{0\%}     & improvement$^\dagger$ \\
Model  &  &  &  &  &  &  & & over $\epsilon_{\text{worst-case}}$ \\
\hline
% MNIST 2$\times${[}20{]}   &     &     &     &    &     &        &    & \\
% MNIST 3$\times${[}20{]}   &     &     &     &    &     &        &    & \\
MNIST 2x{[}1024{]} & 0.02904               & \bf 0.03725 & 0.03819 & 0.03828 & 0.03837 & 0.03849 & 0.04075 & \bf 28.2\% \\
MNIST 3x{[}1024{]} & 0.02082               & \bf 0.02299 & 0.02320 & 0.02322 & 0.02324 & 0.02326 & 0.02410 & \bf 10.4\% \\
MNIST 4x{[}1024{]} & 0.00796               & \bf 0.00817 & 0.00819 & 0.00819 & 0.00819 & 0.00819 & 0.00835 & \bf 2.6\% \\
% CIFAR 5$\times${[}2048{]}   &     &     &     &    &     &        &    & \\
% CIFAR 7$\times${[}1024{]}   &     &     &     &    &     &        &    & \\
\hline
\end{tabular}
\end{subtable}
\vspace{0.4cm}
\begin{subtable}{1\textwidth}
\caption{Input is \textcolor{blue}{general} correlated Gaussian}
\label{subtab:gaussianCORR1}
\begin{tabular}{c|ccccccc|c}
\hline
Indpdt. input $X_i$ & \multirow{2}{*}{$\epsilon_{\text{worst-case}}$} & \multirow{2}{*}{(100 - $\eta$)\% $^\dagger$}  & \multirow{2}{*}{75\%}    & \multirow{2}{*}{50\%}    & \multirow{2}{*}{25\%}    & \multirow{2}{*}{5\%}     & \multirow{2}{*}{0\%}     & improvement$^\dagger$ \\
Model  &  &  &  &  &  &  & & over $\epsilon_{\text{worst-case}}$ \\
\hline
% MNIST 2$\times${[}20{]}   &     &     &     &    &     &        &    & \\
% MNIST 3$\times${[}20{]}   &     &     &     &    &     &        &    & \\
MNIST 2x{[}1024{]} & 0.02904               & \bf 0.03679 & 0.03815 & 0.03828 & 0.03841 & 0.03859 & 0.04075 & \bf 26.6\% \\
MNIST 3x{[}1024{]} & 0.02082               & \bf 0.02287 & 0.02319 & 0.02322 & 0.02324 & 0.02329 & 0.02410 & \bf 9.8\% \\
MNIST 4x{[}1024{]} & 0.00796               & \bf 0.00816 & 0.00819 & 0.00819 & 0.00819 & 0.00819 & 0.00835 & \bf 2.5\% \\
% CIFAR 5$\times${[}2048{]}   &     &     &     &    &     &        &    & \\
% CIFAR 7$\times${[}1024{]}   &     &     &     &    &     &        &    & \\
\hline
\end{tabular}
\end{subtable}
\end{table*}
